# Supplementary material for: Implementation in Advised Strategies: Welfare Guarantees from Posted-Price Mechanisms when Demand Queries are NP-hard
Source: arXiv:1910.04342 source file (2020-08-04)
Supplement: Supplementary file 1 [file old_tikz.tex]

\begin{notshow}
\begin{tikzpicture}[node distance=5cm, semithick, auto] 
	\node[circle, minimum width=0.5cm, inner sep = 0pt, black, draw](l1){};
	\node[below=0.06cm of l1]{\scriptsize$\bm{B_1}$};
	
	\node[circle, minimum width=0.5cm, inner sep = 0pt, black, draw](l2)[right=0.6cm of l1]{};
	\node[below=0.06cm of l2]{\scriptsize$B_2$};
	
	\node[circle, minimum width=0.5cm, inner sep = 0pt, black, draw](l3)[right=0.6cm of l2]{};
	\node[below=0.06cm of l3]{\scriptsize$\bm{B_3}$};

	\node[circle, minimum width=0.5cm, inner sep = 0pt, black, draw](l4)[right=0.6 of l3]{};
	\node[below=0.06cm of l4]{\scriptsize$B_4$};

	\node[circle, minimum width=0.5cm, inner sep = 0pt, black, draw](l5)[right=0.6cm of l4]{};
	\node[below=0.06cm of l5]{\scriptsize$\bm{B_5}$};

	\node[circle, minimum width=0.5cm, inner sep = 0pt, black, draw](l6)[right=0.6cm of l5]{};
	\node[below=0.06cm of l6]{\scriptsize$B_6$};

	\node[circle, minimum width=0.5cm, inner sep = 0pt, black, draw](l7)[right=0.6cm of l6]{};
	\node[below=0.06cm of l7]{\scriptsize$\bm{B_7}$};

	\node[circle, minimum width=0.5cm, inner sep = 0pt, black, draw](l8)[right=0.6cm of l7]{};
	\node[below=0.06cm of l8]{\scriptsize$B_8$};

	
	\draw[opacity=0] (l1) --(l2) node(l12)[midway]{};
	\draw[opacity=0] (l3) --(l4) node(l34)[midway]{};
	\draw[opacity=0] (l5) --(l6) node(l56)[midway]{};
	\draw[opacity=0] (l7) --(l8) node(l78)[midway]{};
	
	
	\node[circle, minimum width=0.5cm, inner sep = 0pt, black, draw](a1)[above =0.75cm of l12]{};
	\node[below left=-0.2cm and 0.05cm of a1]{\scriptsize$(\bm{B_1},B_2)$};
	
	\node[circle, minimum width=0.5cm, inner sep = 0pt, black, draw](a2)[above = 0.75cm of l34]{};
	\node[below left=-0.2cm and 0.05cm of a2]{\scriptsize$(\bm{B_3},B_4)$};
	\node[circle, minimum width=0.5cm, inner sep = 0pt, black, draw](a3)[above = 0.75cm of l56]{};
	\node[below right=-0.2cm and 0.05cm of a3]{\scriptsize$(\bm{B_5},B_6)$};
	\node[circle, minimum width=0.5cm, inner sep = 0pt, black, draw](a4)[above = 0.75cm of l78]{};
	\node[below right=-0.2cm and 0.05cm of a4]{\scriptsize$(\bm{B_7},B_8)$};

	\draw[opacity=0] (a1) --(a2) node(a12)[midway]{};
	\draw[opacity=0] (a3) --(a4) node(a34)[midway]{};
	
	\node[circle, minimum width=0.5cm, inner sep = 0pt, black, draw](b1)[above=0.75cm of a12]{};
	\node[below left=-0.2cm and 0.1cm of b1]{\scriptsize $(\bm{B_1},B_2,\bm{B_3},B_4)$};

	\node[circle, minimum width=0.5cm, inner sep = 0pt, black, draw](b2)[above=0.75cm of a34]{};
	\node[below right=-0.2cm and 0.1cm of b2]{\scriptsize$(\bm{B_5},B_6,\bm{B_7},B_8)$};

	\draw[opacity=0] (b1) --(b2) node(b12)[midway]{};

	\node[circle, minimum width=0.5cm, inner sep = 0pt, black, draw](c1)[above=0.75cm of b12]{};
	\node[above = 0.1cm of c1]{\scriptsize$(\bm{B_1},B_2,\bm{B_3},B_4,\bm{B_5},B_6,\bm{B_7},B_8)$};
	
	\draw
	(l1) -- (a1)
	(l2) -- (a1)
	(l3) -- (a2)
	(l4) -- (a2)
	(l5) -- (a3)
	(l6) -- (a3)
	(l7) -- (a4)
	(l8) -- (a4)
	(a1) -- (b1)
	(a2) -- (b1)
	(a3) -- (b2)
	(a4) -- (b2)
	(b1) -- (c1)
	(b2) -- (c1); 

	
\end{tikzpicture}
\caption{\cite[Figure~2]{AssadiS19} An illustration of a price tree $T$ with $\alpha = 2$ and $\beta = 2$. By constructing the tree over only bold-faced price buckets, we obtain the modified price tree $T^o$.}
\end{notshow}
